# Supplementary material for: TeCoNeRV: Leveraging Temporal Coherence for Compressible Neural Representations for Videos
Source: arXiv:2602.16711 source file (2026-11-01)
Supplement: Supplementary file 1 [file suppl_style.tex]

\makeatletter
\def\bmv@unhbox#1{\expandafter\unhcopy \csname bmv@box #1 \endcsname}

\newcommand{\bmvasupplementarytitle}{%
  \clearpage
  \global\@topnum\z@
  \bmv@strut\\[-4pt]%
  \begin{raggedright}%
    {\bmv@titlesize\bfseries\sffamily\textcolor{bmv@sectioncolor}{\@title}\par}%
    \vskip 0.35em%
    {\bmv@titlesize\bfseries\sffamily\textcolor{bmv@sectioncolor}{Supplementary Material}\par}%
    \vskip 1.5em%
    {\bmv@RenderAuthorsAndInstitutions}%
  \end{raggedright}%
  \vskip\baselineskip
  \hrule
  \vskip\baselineskip
}
\makeatother

\setcounter{tocdepth}{-10} %

\newcommand{\suppltableofcontents}{%
  \begingroup
    \makeatletter
    \colorlet{toclink}{bmv@sectioncolor!80!white}
    \makeatother
    \hypersetup{linkcolor=toclink}%
    \tableofcontents
  \endgroup
}
